# Supplementary material for: That Was Then, This Is Now: A Security Evaluation of Password Generation, Storage, and Autofill in Thirteen Password Managers
Source: arXiv:1908.03296 source file (2019-12-10)
Supplement: Supplementary file 1 [file appendix.tex]

%!TEX root = main.tex

\section{Appendix}\label{sec:appendix}

\subsection{Secure Password Generator}\label{sub:securepasswordgenerator}

Based upon the results of our analysis of password generators we created a secure password generator in python. Our generator can be installed as a python package via the Python Package Index using the command \emph{pip install securepasswordgenerator}. It both provides a command line utility and exposes a generator class that can be imported. 

To avoid generating trivially guessable passwords, we implemented a zxcvbn filter per our suggestion in Section~\ref{sub:zxcvbnanalysis}. We did so by using a while loop to verify that the generated password had a zxcvbn guess number (log10) within a narrow threshold (.1) of the password length. If the password did not meet this criteria, we generated a new one. 

Because the password managers surveyed provided no valid reason for reducing their symbol set size, we maximized our symbol set to increase password entropy. Our symbol set had a total of 95 characters and used the following symbols---\verb|`~!@#$%^&*()-_=+[]\{};:,./<>?\'" ||. Of the password managers we surveyed, the lowest default password length was twelve (LastPass and Dashlane) and the greatest was twenty (1Password). We chose fifteen for our default length because we believe that represents a balance of usability and security. With our default password length of 15, this character set provides an information entropy of 98.5 which would require on average $10^{29}$ guesses. This guess number puts us comfortably above the $10^{15}$ guesses required for offline resistance. Increasing the length further only reduces usability. 

Like most reviewed password generators, we set the minimum number of digits and symbols to one by default. We found this decision rational because passwords often have to fulfill policy requirements with these same minimums. We also made these values configurable and offered users the option to specify a password specification using the letters l,d and s. For example, 'dddddd' could be used to produce a six digit pin.

\begin{figure*}
    \includegraphics[width=.33\textwidth]{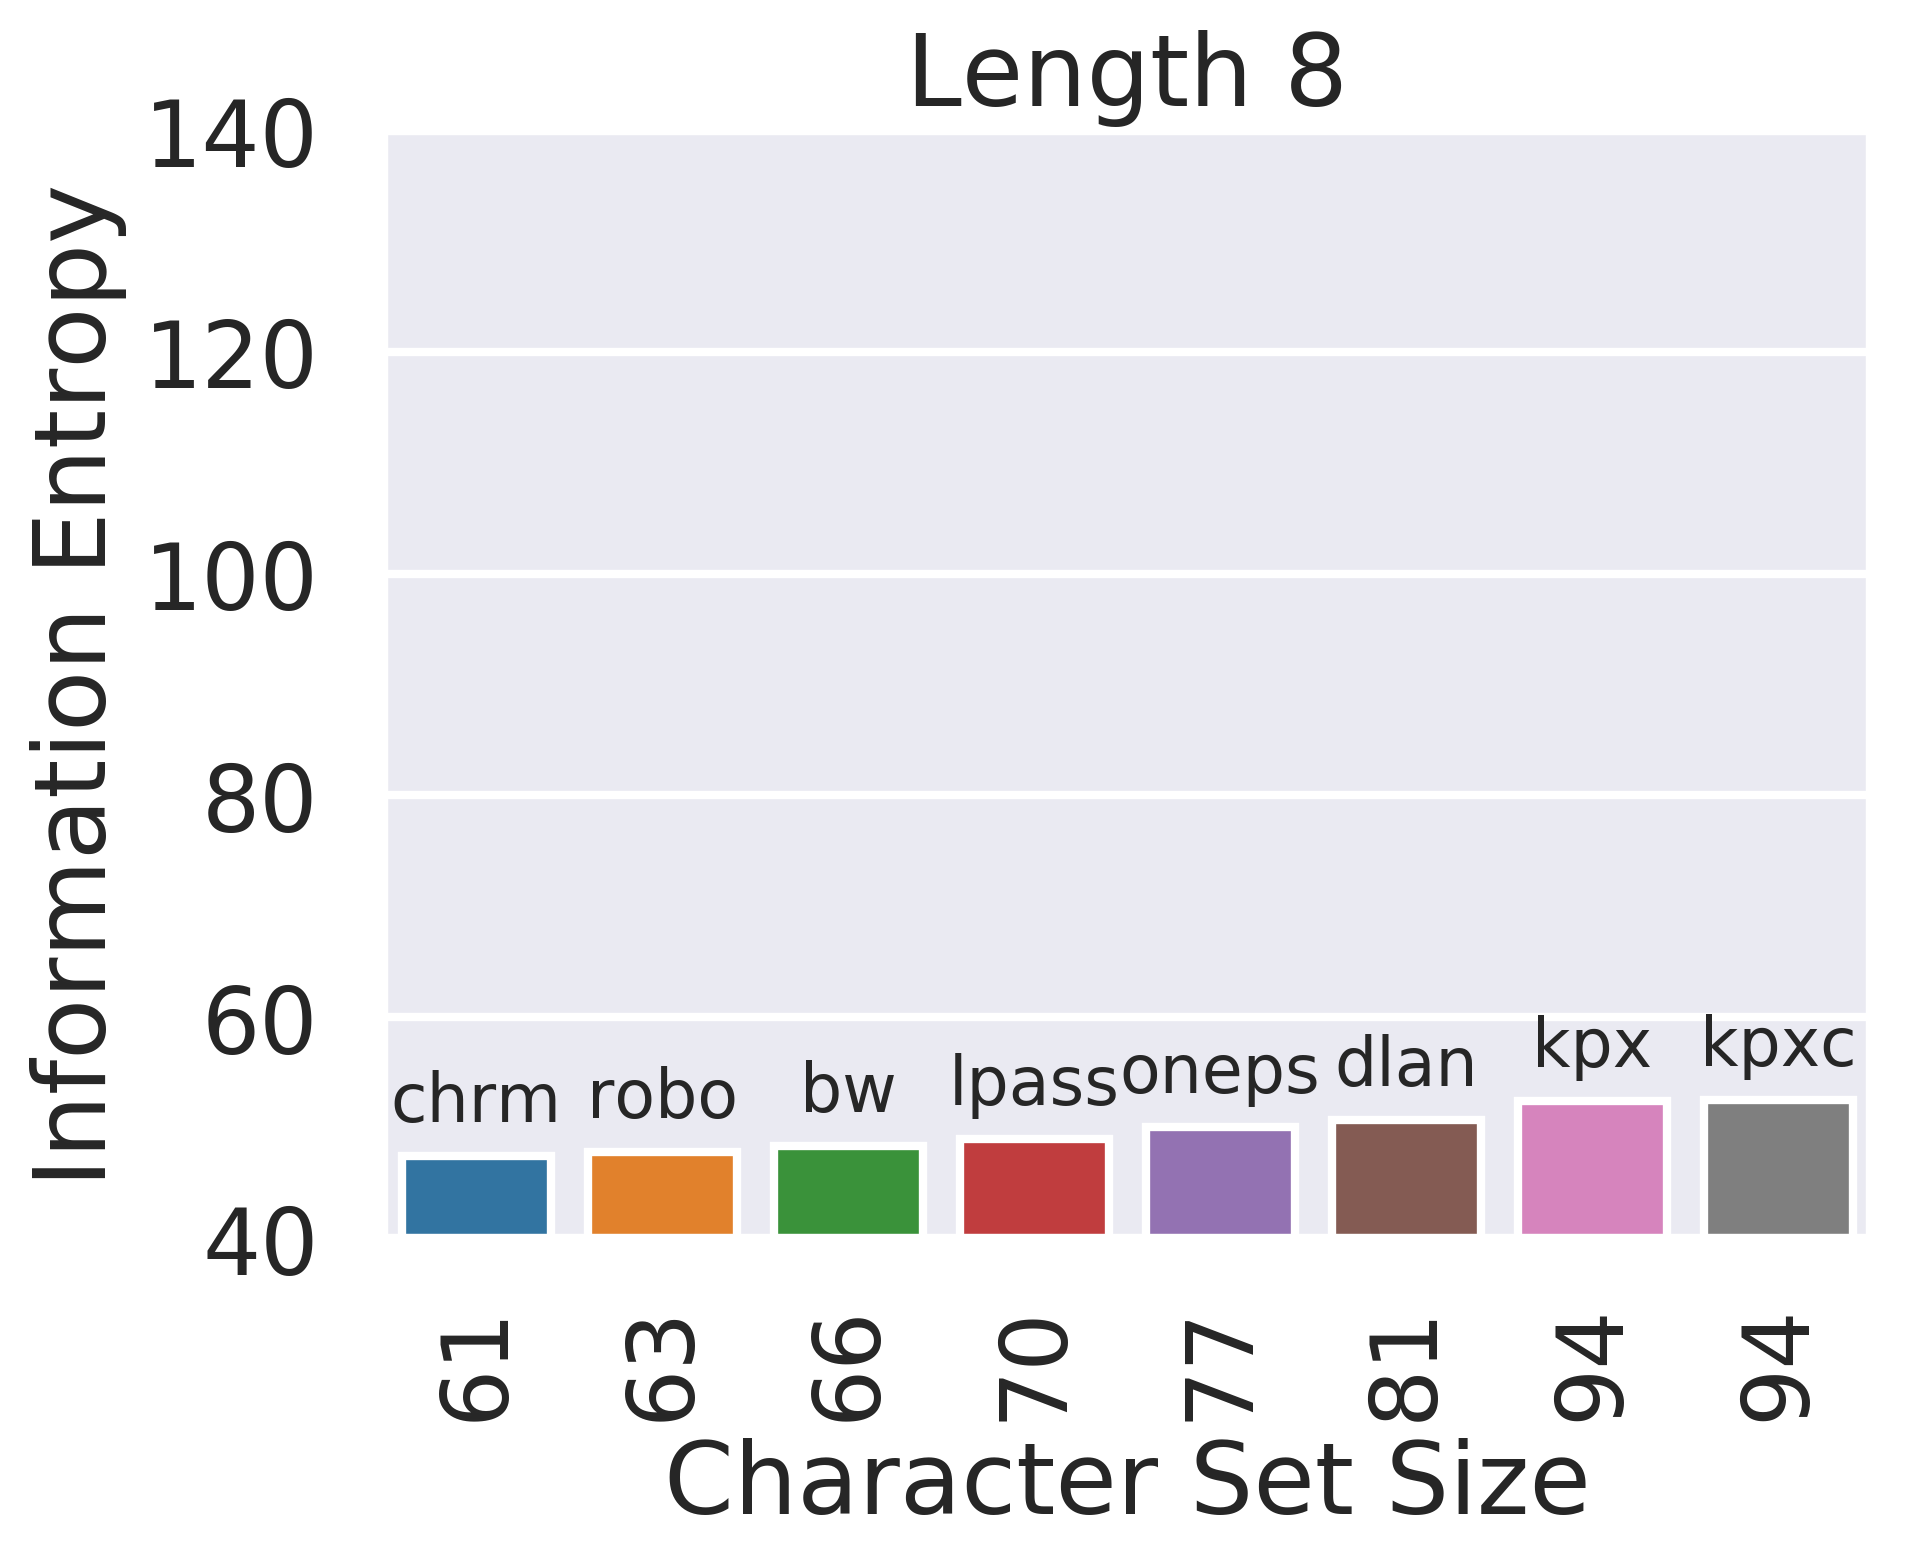}
    \includegraphics[width=.33\textwidth]{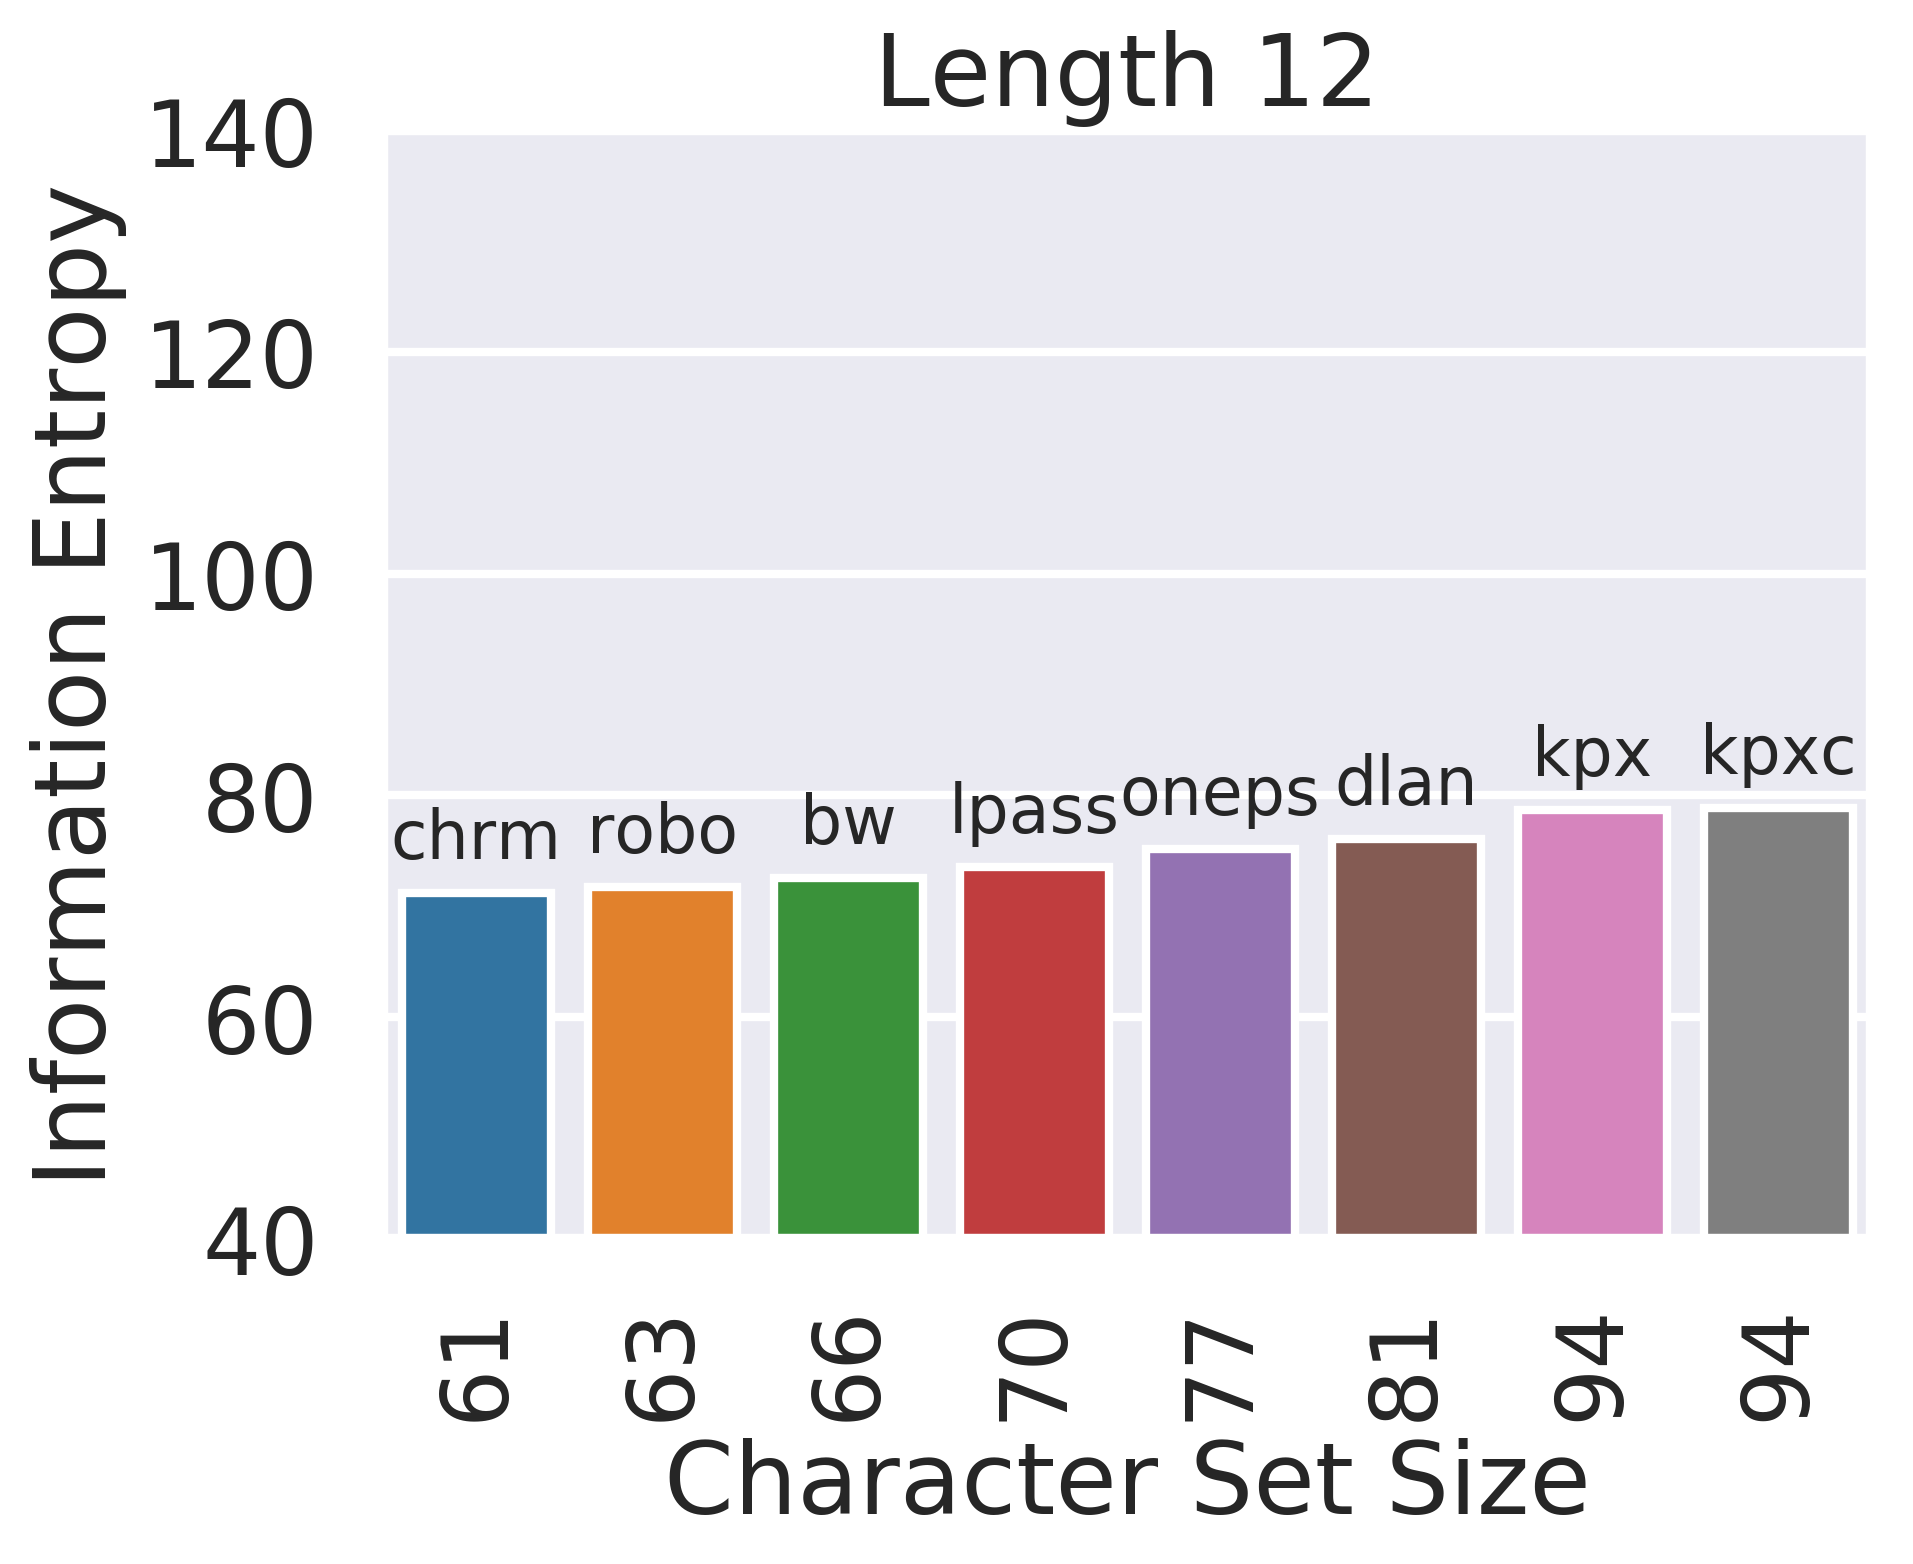}
    \includegraphics[width=.33\textwidth]{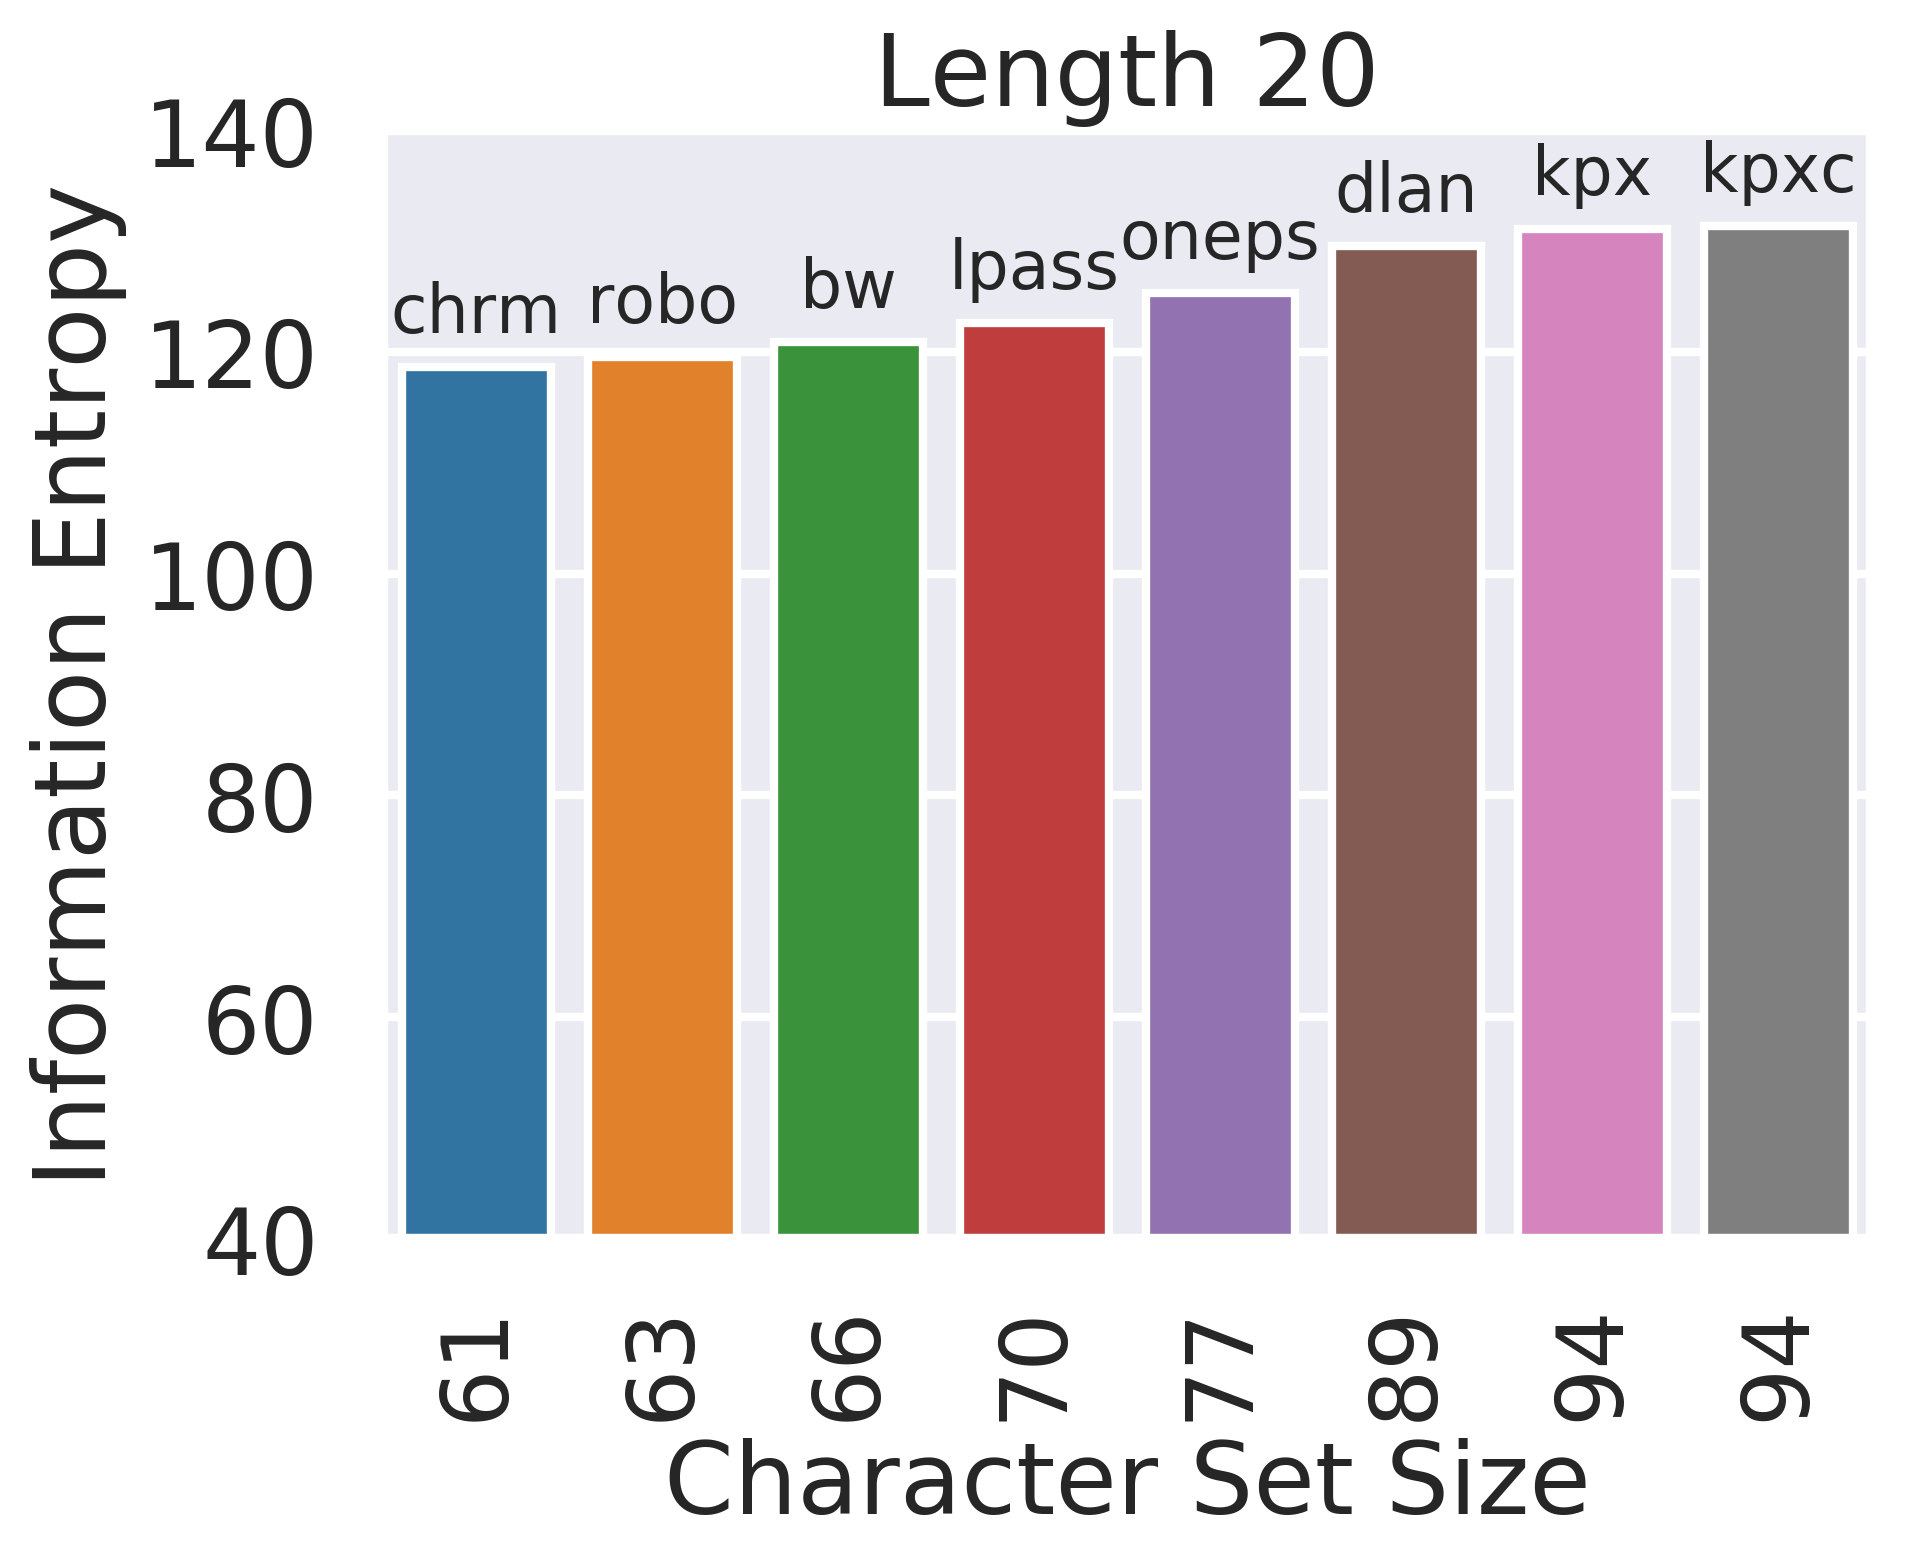}
    \caption{Information Entropy for Password Generators}
    \label{fig:informationentropyall}
\end{figure*}

\begin{figure*}
    \includegraphics[width=.33\textwidth]{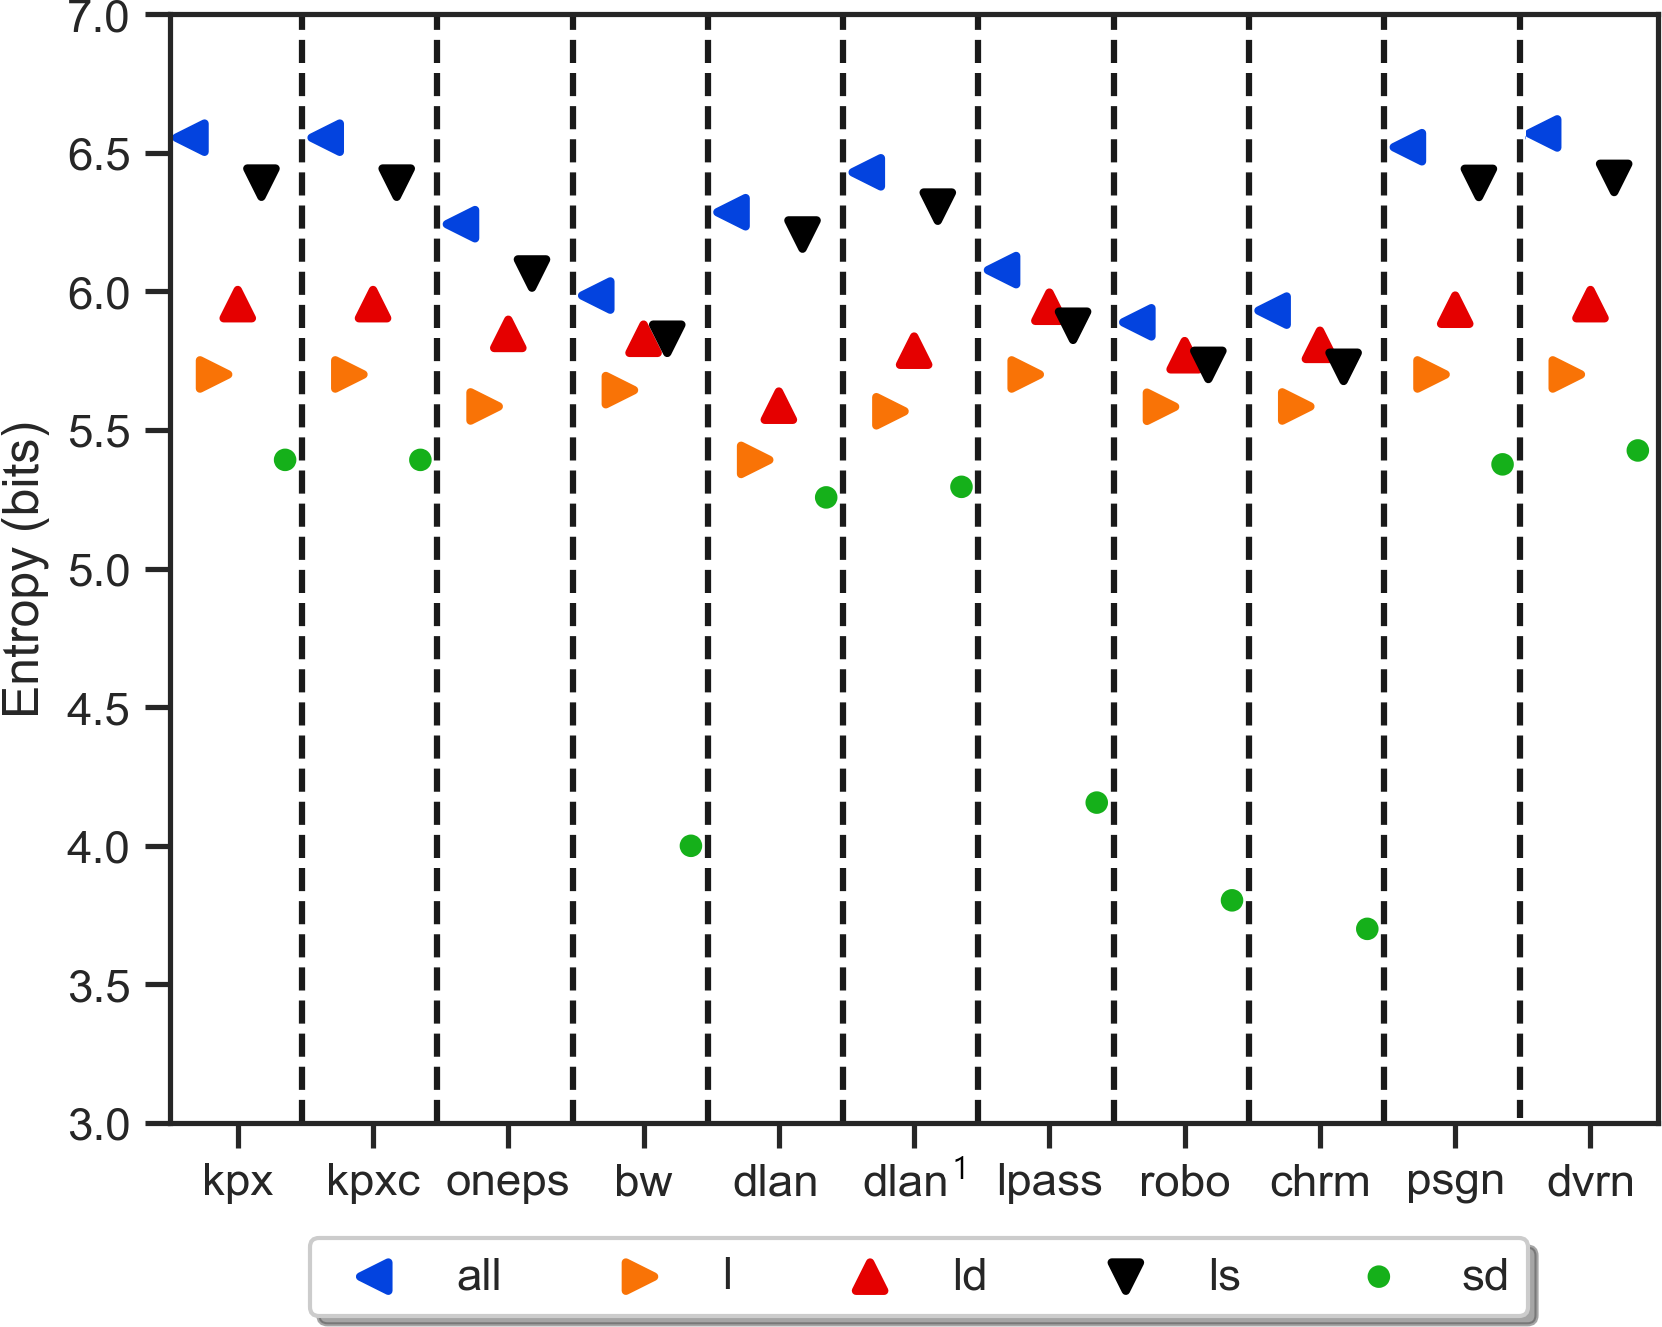}
    \includegraphics[width=.33\textwidth]{Images/genstats/shannon/12shannon_scatter.png}
    \includegraphics[width=.33\textwidth]{Images/genstats/shannon/20shannon_scatter.png}
    \caption{Shannon Entropy for Password Generators}
    \captionsetup{aboveskip=0pt,font=it}
    \caption*{\\Demonstrates that shannon entropy is roughly equivalent across password lengths}
    \label{fig:shannonentropyall}
\end{figure*}

Listing~\ref{lst:blazetrainconfig} and Listing~\ref{lst:blazetestconfig} in the Appendix

\begin{table*}
    \begin{center}
    \begin{tabular}{@{}lGGGGGGGGGGGGGGG@{}}
        & \multicolumn{5}{c}{Length 8} & \multicolumn{5}{c}{Length 12} & \multicolumn{5}{c}{Length 20} \\
        
        \cmidrule(r){2-16}
        \rowcolor{white} 
        & \multicolumn{1}{c}{all} 
        & \multicolumn{1}{c}{l}
        & \multicolumn{1}{c}{ld}
        & \multicolumn{1}{c}{ls} 
        & \multicolumn{1}{c}{sd}
        & \multicolumn{1}{c}{all} 
        & \multicolumn{1}{c}{l}
        & \multicolumn{1}{c}{ld}
        & \multicolumn{1}{c}{ls} 
        & \multicolumn{1}{c}{sd}
        & \multicolumn{1}{c}{all} 
        & \multicolumn{1}{c}{l}
        & \multicolumn{1}{c}{ld}
        & \multicolumn{1}{c}{ls} 
        & \multicolumn{1}{c}{sd}
    \\ \midrule
    \rowcolor{white}
    \textbf{Chrome}                       & 3 & 5 & 4 & 3 & 291 & 5 & 10 & 5 & 5 & 533 & 8 & 19 & 13 & 10 & 1202 \\
    \textbf{RoboForm}                     & 2 & 4 & 4 & 2 & 89 & 6 & 10 & 9 & 5 & 199 & 11 & 18 & 17 & 11 & 533 \\ 
    \rowcolor{white}
    \textbf{LastPass}                     & 1 & 4 & 4 & 2 & 72 & 5 & 9 & 8 & 4 & 248 & 9 & 19 & 15 & 9 & 788 \\                     
    \textbf{Bitwarden}                    & 2 & 5 & 3 & 2 & 51 & 3 & 9 & 7 & 4 & 122 & 9 & 20 & 14 & 8 & 289 \\
    \rowcolor{white}
    \textbf{1Password}                    & 1 & 5 & 4 & 1 & \NA & 1 & 10 & 9 & 2 & \NA & 4 & 17 & 14 & 4 & \NA \\
    \textbf{Dashlane}                     & .8 & 7 & 5 & 1 & 2 & 2 & 13 & 11 & 1 & 5 & 3 & 24 & 17 & 2 & 12 \\
    \rowcolor{white}
    \textbf{KeePassX}                     & 1 & 4 & 5 & 1 & 3 & 1 & 10 & 9 & 1 & 7 & 3 & 21 & 16 & 3 & 11 \\
    \textbf{KeePassXC}                    & 1 & 5 & 4 & 1 & 4 & 2 & 11 & 7 & 1 & 5 & 3 & 20 & 18 & 2 & 13 \\ 
    \rowcolor{white}
    \textbf{PassGen}                      & 1 & 5 & 3 & .5 & 3 & 1 & 8 & 8 & 1 & 8 & 3 & 19 & 15 & 2 & 13 \\
    \textbf{devrandom}                    & .7 & 5 & 4 & 1 & 3 & 2 & 9 & 9 & 2 & 6 & 3 & 19 & 18 & 2 & 10 \\
    \end{tabular}
    \caption{Fraction of Passwords ($e^{-5}$) Below zxcvbn Guess Estimate Threshold}
    \label{tab:fractzxcvbnbelow}
    \captionsetup{aboveskip=0pt,font=it}
    \caption*{\\Threshold for guess estimate is 2 less than the length (ex: for length 8 threshold is 6)}
    \end{center}
\end{table*}

\begin{table*}
    \begin{center}
    \begin{tabular}{@{}lGGGGGG@{}}
        & \multicolumn{2}{c}{Length 8} & \multicolumn{2}{c}{Length 12} & \multicolumn{2}{c}{Length 20} \\
        \rowcolor{white} 
        & \multicolumn{1}{c}{guesses}
        & \multicolumn{1}{c}{password}
        & \multicolumn{1}{c}{guessses}
        & \multicolumn{1}{c}{password}
        & \multicolumn{1}{c}{guesses}
        & \multicolumn{1}{c}{password}
    \\ \midrule
    \rowcolor{white}
    \textbf{chrmall}   & 4.849 & \verb|Tz5a5a5a| & 8.556 & \verb|SNmWQCm4STER|& 16.594 & \verb|ArEiWBJ6g2xFLFLFLYrP|\\
    \rowcolor{white}
    \textbf{chrml}     & 4.773 & \verb|pasSetet| & 8.107 & \verb|sSnfJKnewnew|& 16.283 & \verb|SANDrAyUFHQqzevCzuBV|\\
    \rowcolor{white}
    \textbf{chrmld}    & 5.041 & \verb|guAsEMAj| & 8.602 & \verb|vWT5vWT5hynD|& 16.782 & \verb|4f4f4fb3VFjkAwq4YQu5|\\
    \rowcolor{white}
    \textbf{chrmls}    & 4.716 & \verb|XMXMjnrv| & 8.491 & \verb|ZVRbEttyp:r-||& 16.602 & \verb|hSSzhSSzDcQN:ShLiNfR|\\
    \rowcolor{white}
    \textbf{chrmsd}    & 4.164 & \verb|98449844| & 6.744 & \verb|!:4687687687|& 14.718 & \verb|:8:6.23.9352:9678678|\\
    \textbf{roboall}       & 4.792 & \verb|i#Torr3s| & 8.435 & \verb|GARC!4WNYLk6|& 16.778 & \verb|U5D4ViDnnnVY733D##5!|\\
    \textbf{robol}       & 4.722 & \verb|namesTsT| & 8.75 & \verb|LgaustinwfQA|& 16.272 & \verb|uWDouWDoonmEVosXabFL|\\
    \textbf{robold}       & 5.057 & \verb|iQMWhi7e| & 8.984 & \verb|M4keH4veitXT|& 16.477 & \verb|XqnNfCqWER7YcYDptZMf|\\
    \textbf{robols}       & 5.017 & \verb|SAWyE@rS| & 9.0 & \verb|$Mith$tHDsUY|& 16.079 & \verb|wqmMgV^JagV^JayonTCC|\\
    \textbf{robosd}       & 4.062 & \verb|2345678#| & 6.467 & \verb|2472324723%^|& 15.079 & \verb|66467#9@994!9@994!5^|\\
    \rowcolor{white}
    \textbf{bwall}       & 4.124 & \verb|d@rKn3s5| & 9.0 & \verb|#hUGwH5Sm!Th|& 16.968 & \verb|b4!7eyc&Cr&PnYUiMX9#|\\
    \rowcolor{white}
    \textbf{bwl}       & 4.301 & \verb|NUaeiaei| & 8.093 & \verb|uuaPNLHisHis|& 16.477 & \verb|YyXfBRmfIUZparkerFuP|\\
    \rowcolor{white}
    \textbf{bwld}       & 5.041 & \verb|davI5gxu| & 8.579 & \verb|nEWdEuFsmi7h|& 16.666 & \verb|8UTT6pBihnHCVSJH77ps|\\
    \rowcolor{white}
    \textbf{bwls}       & 4.763 & \verb|w!LSonrV| & 8.5 & \verb|mgzSQx^ad^ad|& 16.38 & \verb|gJSFBf#L$%Lh&esamueL|\\
    \rowcolor{white}
    \textbf{bwsd}       & 4.235 & \verb|98******|  & 7.301 & \verb|!3785!3785!7|& 14.778 & \verb|7^294!5!5!5!54%323&&|\\
    \textbf{lpassall}       & 4.301 & \verb|dP*ydP*y| & 8.922 & \verb|B@KeRee22241|& 16.38 & \verb|daN!elXRy*xqGW*tPDqN|\\
    \textbf{lpassl}       & 4.888 & \verb|VIsAndrA| & 8.782 & \verb|ZdfTirlwlwlw|& 16.623 & \verb|GxEQPSISCQZamfThoMas|\\
    \textbf{lpassld}       & 4.763 & \verb|ax7H0M4s| & 8.403 & \verb|wOWwOWa3Yeht|& 16.651 & \verb|GI6wfznZMlE74JJU5TIN|\\
    \textbf{lpassls}       & 4.849 & \verb|M%M%M%bK| & 8.602 & \verb|*WsteveN@cxi|& 16.477 & \verb|F@mmIllerkqMZc!Fr#T#|\\
    \textbf{lpasssd}       & 4.255 & \verb|####1937| & 7.587 & \verb|^8^806131755|& 14.461 & \verb|@$@$99120015*130!!42|\\
    \rowcolor{white}
    \textbf{onepsall}       & 4.984 & \verb|A78ERT%d| & 8.602 & \verb|wN0swN0s=BLq|& 16.879 & \verb|Z+XTrEbor*U=:0%rA,Es|\\
    \rowcolor{white}
    \textbf{onepsl}       & 4.618 & \verb|yPyPyPCD| & 8.602 & \verb|CPFrCPFrYDWt|& 15.477 & \verb|mZAzKennethDLnYaJfQT|\\
    \rowcolor{white}
    \textbf{onepsld}       & 4.849 & \verb|Z8Z8Z8XA| & 8.76 & \verb|e3QbJpMA57eR|& 15.94 & \verb|zpTaAnRiz35u5anLeriC|\\
    \rowcolor{white}
    \textbf{onepsls}       & 5.041 & \verb|dAvisk~A| & 8.76 & \verb|oMMMMMMT?m*m|& 16.879 & \verb|eJ!eD!trEboRG)u+WcqB|\\
    \textbf{dlanall}       & 5.384 & \verb|zLaN6eL@| & 9.076 & \verb|Q"Q"5o5o>?;E|& 17.075 & \verb|Fj{MgVZ+5?}3%MAs7ERw|\\
    \textbf{dlanl}       & 4.301 & \verb|ADzyxzyx| & 8.639 & \verb|hJQEAaromero|& 15.971 & \verb|JNRRPPkmyTtrebortjfk|\\
    \textbf{dlanld}       & 4.354 & \verb|787878Cx|& 8.17 & \verb|E9NXYMAreAre| & 15.486 & \verb|it5pgXNPXMtG7ZMtG7ZY|\\
    \textbf{dlanls}       & 5.041 & \verb|?Arroger| & 8.782 & \verb|_S@yy}SxSxSx|& 17.0 & \verb|wc[([d_^r~G%wnjbriaN|\\
    \textbf{dlansd}       & 4.480 & \verb|////$8$8| & 8.602 & \verb|{%8&{%8&6)>||& 16.602 & \verb|`*@=<||\verb|-||\verb|[>>~%7[.%7[.|\\
    \rowcolor{white}
    \textbf{kpxall}       & 5.586 & \verb|-#dy3ar$| & 9.48 & \verb|j||\verb|gg1in6(&mR|& 16.977 & \verb|WT||\verb|=6?FOq[nglqglq;=Y|\\
    \rowcolor{white}
    \textbf{kpxl}       & 4.957 & \verb|TaKEdeen| & 8.849 & \verb|MwMwIFUHdodo|& 16.158 & \verb|xSxWgLhtKNpBOammmmmm|\\
    \rowcolor{white}
    \textbf{kpxld}       & 5.013 & \verb|VbI75I75| & 8.732 & \verb|Yq0Yk5j0sEpH|& 16.673 & \verb|YTOJDc7arke02ZXBlkPi|\\
    \rowcolor{white}
    \textbf{kpxls}       & 5.271 & \verb|+H||\verb|SpecK| & 8.837 & \verb|TApVwONKl!kE|& 17.049 & \verb|&jmh;~:^Yd'iaz:M@rIA|\\
    \rowcolor{white}
    \textbf{kpxsd}       & 5.113 & \verb|+++++}67| & 8.782 & \verb|%$%$%$:>%9]0|& 16.477 & \verb|,+#0/.-,+8-*;5/6'8:7|\\
    \textbf{kpxcall}       & 5.041 & \verb|XJkSM!TH| & 9.146 & \verb|AiRAMsQ`p;U[|& 16.385 & \verb|6*)J@M35E>E>mfg5GjUr|\\
    \textbf{kpxcl}       & 4.812 & \verb|lIkeyYyY| & 8.494 & \verb|DGJMPSibhYym|& 16.452 & \verb|TUOBAKrjlwpJOComAkeS|\\
    \textbf{kpxcld}       & 5.041 & \verb|5U5andtL| & 8.623 & \verb|andrEwGR8X5k|& 16.477 & \verb|e5dOkdZwlTAY7ORlv9i9|\\
    \textbf{kpxcls}       & 5.041 & \verb|joNe$bK(| & 9.0 & \verb|nEUAeHvl!NDA|& 17.011 & \verb|(aN'TdnAmFlwf*v@h}$#|\\
    \textbf{kpxcsd}       & 4.848 & \verb|'+'+'+_+| & 8.535 & \verb|!!<!!<\5\5?'|& 15.778 & \verb|468-`[:-`[:(-@6>7+_3|\\
    \rowcolor{white}
    \textbf{psgnall}       & 5.269 & \verb|=,Rl3w1s| & 9.531 & \verb|J7||\verb|nD@&LS\?f|& 16.899 & \verb|OKAYrgO5>f`VGk9si'||\verb|||\verb||\\
    \rowcolor{white}
    \textbf{psgnl}       & 4.301 & \verb|mjBOmjBO| & 8.0 & \verb|CZttOFwIlson|& 16.519 & \verb|SROLYATCytZWzyAikvCN|\\
    \rowcolor{white}
    \textbf{psgnld}       & 4.593 & \verb|GARcI4g0| & 8.283 & \verb|2hY1L5diddid|& 15.477 & \verb|Eiool2bletm3in3JV3rR|\\
    \rowcolor{white}
    \textbf{psgnls}       & 5.322 & \verb|nW$nW$RR| & 9.0 & \verb|?S!eJ'Nsusan|& 17.0 & \verb|(e||\verb|MC>]bQh@j:Sed@VID|\\
    \rowcolor{white}
    \textbf{psgnsd}       & 4.848 & \verb|!0!0!04^| & 8.576 & \verb|',~=85\?\?\?|& 16.0 & \verb|.6#'{0]?58%,!805:05:|\\
    \textbf{dvrnall}       & 5.613 & \verb|g\>LI>LI| & 9.0 & \verb|Nan<yE~XWQAg|& 17.227 & \verb|4lP8HT6R+he||\verb|mAOW5Era|\\
    \textbf{dvrnl}       & 4.584 & \verb|Tesallad| & 9.0 & \verb|MrKNxQNDAViS|& 16.5 & \verb|MpSoeLYMjVLTcdbglbgl|\\
    \textbf{dvrnld}       & 4.301 & \verb|RTRHRTRH| & 8.602 & \verb|9Em29Em2RIN8|& 16.221 & \verb|G7qc02OTUm5DnOSnHOjx|\\
    \textbf{dvrnls}       & 5.037 & \verb|KnoWneee| & 8.584 & \verb|g_||\verb|:KKd@niE||\verb||& 17.079 & \verb|J->xkRTd`Bod`BoL XjM|\\
    \textbf{dvrnsd}       & 4.465 & \verb|31_22_06| & 9.079 & \verb|68=[12?77777|& 16.782 & \verb|?][3[25>81}#+%9(9(9(|\\
    \\ \bottomrule
    \end{tabular}
    \caption{Passwords with Lowest zxcvbn Guess Estimates in Each Category}
    \captionsetup{aboveskip=0pt,font=it}
    \caption*{\\Normal zxcvbn value of log10(guesses) for each length are approximately 8, 12 and 20}
    \label{tab:zxcvbnlow}
    \end{center}
\end{table*}
