# Supplementary material for: That Was Then, This Is Now: A Security Evaluation of Password Generation, Storage, and Autofill in Thirteen Password Managers
Source: arXiv:1908.03296 source file (2019-12-10)
Supplement: Supplementary file 2 [file autofill-appendix.tex]

%!TEX root = main.tex

\section{Additional Autofill Data}
\label{appx:autofill}

\begin{appxitem}
	\begin{lstlisting}[language=csp,captionpos=b,caption=Content Security Policy---1Password X,label=lst:csp-1passwordx]
	default-src 'none';
	script-src https://js.stripe.com https://app.1password.com;
	connect-src 'self' https://watchtower.1password.com https://api.pwnedpasswords.com https://api.stripe.com https://app.1password.com wss://b5n.1password.com https://f.1passwordusercontent.com/ *.1password.com https://*.1password.ca https://*.1password.eu https://*.ent.1password.com;
	child-src 'self' https://js.stripe.com;
	form-action 'none';
	frame-src 'self' https://js.stripe.com https://*.duosecurity.com;
	img-src data: blob: https://c.1password.com https://app.1password.com https://a.1passwordusercontent.com/ https://a.1passwordusercontent.ca https://a.1passwordusercontent.eu https://a.1passwordentusercontent.com;
	report-uri https://my.1password.com/csp_violation;
	style-src https://app.1password.com;
	\end{lstlisting}
\end{appxitem}
\vspace{-.2cm}

\begin{appxitem}
	\begin{lstlisting}[language=csp,captionpos=b,caption=Content Security Policy---Bitwarden,label=lst:csp-bitwarden]
	default-src 'self';
	script-src 'self' 'sha256-ryoU+5+IUZTuUyTElqkrQGBJXr1brEv6r2CA62WUw8w=' https://js.stripe.com https://js.braintreegateway.com https://www.paypalobjects.com;
	object-src 'self' blob:;
	child-src 'self' https://js.stripe.com https://assets.braintreegateway.com https://*.paypal.com https://*.duosecurity.com;
	connect-src 'self' wss://notifications.bitwarden.com https://notifications.bitwarden.com https://cdn.bitwarden.net https://api.pwnedpasswords.com https://twofactorauth.org https://api.stripe.com https://www.paypal.com https://api.braintreegateway.com https://client-analytics.braintreegateway.com https://*.braintree-api.com;
	frame-src 'self' https://js.stripe.com https://assets.braintreegateway.com https://*.paypal.com https://*.duosecurity.com;
	img-src 'self' data: https://icons.bitwarden.net https://*.paypal.com https://www.paypalobjects.com https://q.stripe.com https://haveibeenpwned.com https://www.gravatar.com;
	style-src 'self' 'unsafe-inline' https://assets.braintreegateway.com https://*.paypal.com;
	\end{lstlisting}
\end{appxitem}

\begin{appxitem}
	\begin{lstlisting}[language=csp,captionpos=b,caption=Content Security Policy---Dashlane,label=lst:csp-dashlane]
	default-src 'none';
	script-src 'self' 'unsafe-eval' https://d1sk9wm475w15q.cloudfront.net;
	object-src 'none';
	base-uri 'none';
	block-all-mixed-content;
	child-src 'self' blob:;
	connect-src 'self' https://ws1.dashlane.com https://logs.dashlane.com https://www.dashlane.com https://api.stripe.com https://kck3hlb9.dashlane.com https://api.dashlane.com https://wstests.dashlane.com:* ;
	font-src data: https://fonts.gstatic.com;
	frame-ancestors 'none';
	frame-src https://d1sk9wm475w15q.cloudfront.net;
	img-src data: https://d1sk9wm475w15q.cloudfront.net https://d2erpoudwvue5y.cloudfront.net https://static-icons.s3-eu-west-1.amazonaws.com https://gravatar.com;
	report-uri https://kck3hlb9.dashlane.com/1/csp-report/create;
	style-src 'unsafe-inline' https://fonts.googleapis.com;
	\end{lstlisting}
\end{appxitem}

\begin{appxitem}
	\begin{lstlisting}[language=csp,captionpos=b,caption=Content Security Policy---LastPass,label=lst:csp-lastpass]
	default-src 'self';
	script-src 'self' 'unsafe-inline' 'unsafe-eval';
	object-src 'self';
	connect-src 'self' https://lastpass.com https://pollserver.lastpass.com https://loglogin.lastpass.com https://accounts.lastpass.com https://login.microsoftonline.com https://graph.microsoft.com https://provisioning-api-prod.service.lastpass.com;
	font-src data: 'self' 'unsafe-inline' 'unsafe-eval' https://lastpass.com;
	frame-src 'self' https://cdn.lmiutil.com https://*.duosecurity.com
	img-src 'self' data: https://*.google-analytics.com https://lastpass.com https://analytics.twitter.com/i/adsct https://www.facebook.com/tr https://lp-cdn.lastpass.com;
	plugin-types application/x-invalid-type;
	style-src 'self' 'unsafe-inline' 'unsafe-eval' https://lastpass.com;
	\end{lstlisting}
\end{appxitem}
